# Supplementary material for: Implications of Annotation Artifacts in Edge Probing Test Datasets
Source: arXiv:2310.13856 source file (2023-10-20)
Supplement: Supplementary file 1 [file supplementary.tex]

\section*{Appendix}
In the following results, M. stands for mean and W. stands for weighted. Mcc. stands for Matthews Correlation Coefficient.

% Filters
\newcommand{\nofilter}{No Filter}
\newcommand{\random}{Mem-Unif}
\newcommand{\trndist}{Mem-Freq}
\newcommand{\trninput}{Mem-Ex} % any better name?

% probes

\newcommand{\bbl}{Bert base cased, linear}
\newcommand{\bblr}{Bert base cased, linear, random}
\newcommand{\rbl}{Roberta base, linear}
\newcommand{\rblr}{Roberta base, linear, random}
\newcommand{\bbm}{Bert base cased, mlp}
\newcommand{\bbmr}{Bert base cased, mlp, random}
\newcommand{\rbm}{Roberta base, mlp}
\newcommand{\rbmr}{Roberta base, mlp, random}

% metrics
\newcommand{\acc}{Accuracy}
\newcommand{\wtdprec}{W. Prec}
\newcommand{\wtdrec}{W. Recall}
\newcommand{\wtdf}{W. F1}
\newcommand{\meanrec}{M. Recall}
\newcommand{\macrof}{Macro F1}
\newcommand{\meanprec}{M. Prec}

%spacing
\newcommand\Tstrut{\rule{0pt}{2.6ex}}         % = `top' strut
   % = `bottom' strut

\newcommand{\segment}[1]{
&\nofilter &\multicolumn{7}{r}{\multirow{4}{*}{\begin{tabularx}{0.6\textwidth}{XXXXXXX}#1\end{tabularx}}}\Tstrut \\
&\random &\multicolumn{7}{X}{} \\
&\trndist &\multicolumn{7}{X}{} \\
&\trninput &\multicolumn{7}{X}{} \\
}

\newcommand{\myTable}[9]{
\begin{table}[H]
\centering
\scriptsize
\begin{tabular}{llrrrrrrrr}\toprule
Probe &Filter&
\multicolumn{7}{}{\multirow{1}{*}{
\begin{tabularx}{0.6\textwidth}{XXXXXXX}\acc&\wtdprec &\wtdrec & \wtdf & \meanrec & \macrof &\meanprec \end{tabularx}
}}\\
\midrule
\multirow{4}{*}{\bbl}
\segment{#1}
\hline
\multirow{4}{*}{\bblr}
\segment{#2}
\hline
\multirow{4}{*}{\rbl}
\segment{#3}
\hline
\multirow{4}{*}{\rblr}
\segment{#4}
\hline
\multirow{4}{*}{\bbm}
\segment{#5}
\hline
\multirow{4}{*}{\bbmr}
\segment{#6}
\hline
\multirow{4}{*}{\rbm}
\segment{#7}
\hline
\multirow{4}{*}{\rbmr}
\segment{#8}

\bottomrule
\end{tabular}
\caption{#9 test results}
\label{tab:example2}
\end{table}
}

\myTable{96.83 &96.8 &96.83 &96.81 &54.16 &54.19 &54.26 \\
93.38 &93.28 &93.38 &93.31 &51.79 &51.77 &51.85 \\
96.22 &96.18 &96.22 &96.19 &52.24 &52.23 &52.33 \\
87.96 &87.83 &87.96 &87.81 &45.9 &45.49 &45.49 \\}{82.8 &74.1 &82.8 &76.96 &15.65 &16.54 &23.03 \\
71.94 &60.22 &71.94 &62.22 &14.98 &14.83 &22.88 \\
80.79 &71.16 &80.79 &74.46 &15.6 &16.35 &22.17 \\
54.26 &44.76 &54.26 &41.12 &14.2 &12.08 &20.2 \\}{97.01 &97.06 &97.01 &97.01 &55.04 &54.45 &54.04 \\
93.64 &93.74 &93.64 &93.63 &52.35 &51.69 &51.27 \\
96.45 &96.53 &96.45 &96.46 &53.37 &52.68 &52.21 \\
88.65 &88.89 &88.65 &88.65 &47.11 &45.93 &45.33 \\}{82.58 &74.19 &82.58 &76.63 &15.27 &16.01 &23.94 \\
71.86 &60.92 &71.86 &62.06 &14.8 &14.59 &24.13 \\
80.61 &71.38 &80.61 &74.17 &15.18 &15.83 &23.72 \\
54.42 &47.28 &54.42 &41.36 &14.06 &11.87 &22.78 \\}{96.94 &97.1 &96.94 &96.98 &55.44 &54.35 &53.58 \\
92.99 &93.35 &92.99 &93.08 &52.33 &51.12 &50.33 \\
96.36 &96.58 &96.36 &96.43 &54 &52.68 &51.72 \\
86.6 &87.76 &86.6 &87.03 &46.71 &44.94 &43.83 \\}{85.03 &82.58 &85.03 &80.55 &20.99 &24.35 &44.93 \\
75.22 &74.13 &75.22 &68.34 &20.92 &23.62 &44.8 \\
82.64 &78.96 &82.64 &77.35 &19.15 &21.65 &38.86 \\
57.34 &60.12 &57.34 &47.55 &16.7 &16.32 &34.58 \\}{97.46 &97.52 &97.46 &97.48 &56.29 &55.58 &55.04 \\
94.35 &94.46 &94.35 &94.38 &53.75 &53 &52.4 \\
96.99 &97.06 &96.99 &97.01 &54.89 &54.1 &53.48 \\
89.44 &89.77 &89.44 &89.53 &48.77 &47.6 &46.75 \\}{84.7 &83.11 &84.7 &80.15 &20.19 &23.65 &48.56 \\
74.79 &75.15 &74.79 &67.6 &19.74 &22.33 &48.43 \\
82.68 &80.32 &82.68 &77.47 &18.91 &21.42 &43.09 \\
58.14 &61.11 &58.14 &48.82 &17.25 &17.18 &34.75\\}{\conllner}

\myTable{92.93 &93.55 &92.93 &93.03 &83.64 &83.08 &85.45 \\
89.27 &90.18 &89.27 &89.34 &80.25 &80.56 &84.72 \\
92.63 &93.06 &92.63 &92.67 &81.96 &81.39 &83.84 \\
87.95 &88.67 &87.95 &87.93 &77.05 &76.76 &81.42 \\
}{50.68 &66.1 &50.68 &52.77 &38.73 &40.47 &67.91 \\
48.07 &61.92 &48.07 &47.93 &35.35 &36.57 &67.01 \\
43.09 &57.83 &43.09 &43.74 &29.37 &28.99 &56.97 \\
35.83 &46.73 &35.83 &33.48 &20.78 &18.85 &35.78 \\}{93.91 &94.36 &93.91 &93.96 &84.94 &85.9 &89.58 \\
90.48 &91.29 &90.48 &90.57 &82.57 &83.68 &87.76 \\
93.42 &93.87 &93.42 &93.45 &82.96 &83.5 &87.32 \\
88.83 &89.64 &88.83 &88.86 &77.02 &76.47 &77.71 \\}{49.62 &62.24 &49.62 &50.92 &37.09 &39.54 &63.95 \\
47 &56.66 &47 &45.97 &34.04 &35.51 &60.09 \\
42.39 &53.75 &42.39 &42.5 &26.3 &26.2 &51.44 \\
35.11 &38.23 &35.11 &33.29 &18.96 &17.05 &21.52 \\}{89.33 &92.58 &89.33 &89.82 &79.44 &78.11 &83.35 \\
85.37 &89.38 &85.37 &85.8 &76.59 &76.4 &83.48 \\
89.79 &91.44 &89.79 &89.8 &76.97 &75.53 &77.75 \\
84.55 &86.02 &84.55 &84.3 &70.77 &69.68 &73.22 \\}{59.71 &72.33 &59.71 &60.43 &37.47 &41.75 &63.58 \\
54.71 &65.39 &54.71 &53.19 &33.09 &36.89 &61.93 \\
51.76 &63.98 &51.76 &50.6 &28.47 &32.32 &49.13 \\
38.53 &37.78 &38.53 &30.1 &15.59 &16.4 &29.12 \\}{91.55 &93.42 &91.55 &91.95 &83.71 &82.14 &85.29 \\
87.49 &90.01 &87.49 &87.92 &80.93 &79.72 &84.01 \\
92.5 &93.34 &92.5 &92.56 &82.07 &80.57 &80.91 \\
87.38 &88.46 &87.38 &87.3 &75.93 &74.18 &75.03 \\}{59.05 &70.95 &59.05 &59.78 &40.22 &44.82 &66.82 \\
54.9 &64.75 &54.9 &53.82 &36.75 &41.38 &65.02 \\
52.3 &63.77 &52.3 &51.04 &30.49 &34.02 &58.77 \\
41.77 &42.88 &41.77 &34.83 &18.88 &20.48 &38.22 \\}{\ontonotesner}

\myTable{96.54 &96.58 &96.54 &96.54 &92.97 &92.42 &92.53 \\
96.41 &96.42 &96.41 &96.4 &89.36 &89.62 &90.41 \\
93.87 &94.04 &93.87 &93.85 &88.39 &87.48 &89.24 \\
81.62 &81.47 &81.62 &81.14 &35.01 &32.17 &32.25 \\}{62.04 &76.46 &62.04 &58.77 &58.25 &60.22 &77.69 \\
67.92 &80.47 &67.92 &65.93 &53.51 &56.14 &75.21 \\
38.27 &49.65 &38.27 &29.65 &46.11 &44.98 &61.42 \\
17.43 &28.17 &17.43 &7.26 &3.53 &1.67 &3.53 \\}{96.99 &97 &96.99 &96.98 &93.54 &93.41 &93.9 \\
96.79 &96.8 &96.79 &96.78 &90.55 &90.71 &91.91 \\
94.52 &94.55 &94.52 &94.43 &88.57 &88.29 &90.52 \\
83.3 &82.62 &83.3 &82.66 &40.99 &37.45 &36.63 \\}{61.17 &79.26 &61.17 &57.76 &57.68 &59.45 &79.55 \\
67.5 &82.44 &67.5 &65.28 &52.62 &54.25 &72.77 \\
36.34 &49 &36.34 &26.97 &43.1 &41.33 &60.05 \\
17.29 &24.71 &17.29 &5.86 &2.08 &0.78 &1.89 \\}{97.34 &97.38 &97.34 &97.35 &93.72 &92.71 &92.4 \\
97.05 &97.08 &97.05 &97.05 &88.81 &87.99 &87.91 \\
95.15 &95.26 &95.15 &95.13 &89.18 &88.1 &89.23 \\
82.98 &83.03 &82.98 &82.69 &36.17 &33.34 &33.21 \\}{79.95 &83.55 &79.95 &79.89 &68.16 &69.49 &75.41 \\
82.3 &84.77 &82.3 &82.23 &63.35 &64.92 &71.85 \\
60.36 &67.05 &60.36 &59.13 &56.94 &56.36 &65.49 \\
27.98 &37.61 &27.98 &24.74 &8.59 &7.74 &11.24 \\}{97.45 &97.48 &97.45 &97.45 &92.44 &91.41 &90.86 \\
97.3 &97.32 &97.3 &97.3 &89.84 &89.32 &89.22 \\
95.06 &95.15 &95.06 &95.03 &87.11 &86.19 &86.64 \\
84.17 &83.98 &84.17 &83.81 &38.54 &36.11 &35.85 \\}{78.12 &83.61 &78.12 &78.76 &68.07 &69.97 &78.9 \\
80.99 &85.33 &80.99 &81.58 &63.03 &64.17 &72.46 \\
56.26 &65.32 &56.26 &55.1 &51.96 &51.31 &65.46 \\
40.82 &33.51 &40.82 &29.82 &4.39 &4.18 &6.36 \\}{\ontonotespos}

\myTable{94.38 &94.35 &94.38 &94.35 &91.58 &92.02 &92.69 \\
92.96 &92.92 &92.96 &92.91 &89.72 &90.14 &90.82 \\
92.07 &92.09 &92.07 &92.04 &88.18 &88.36 &88.9 \\
79.74 &80.34 &79.74 &79.78 &65.49 &62.33 &66.4 \\}{63.47 &65.34 &63.47 &60.18 &57.35 &56.45 &70.26 \\
65.31 &67.29 &65.31 &62.58 &55.93 &55.01 &63.93 \\
52.25 &48.45 &52.25 &46.1 &43.21 &41.84 &56.93 \\
25.93 &13.06 &25.93 &15.78 &14.41 &10.7 &13.66 \\}{95.51 &95.5 &95.51 &95.49 &92.97 &93.29 &93.81 \\
94.12 &94.1 &94.12 &94.08 &90.79 &91.24 &92.09 \\
93.65 &93.7 &93.65 &93.63 &90.15 &90.22 &90.8 \\
83.71 &83.88 &83.71 &83.58 &79.04 &74.51 &73.78 \\}{62.14 &64.65 &62.14 &59.04 &55.34 &54.87 &69.64 \\
63.93 &66.05 &63.93 &61.31 &54.4 &53.78 &62.4 \\
51.24 &47.84 &51.24 &45.75 &41.79 &40.07 &51.09 \\
24.61 &10.85 &24.61 &15.02 &8.76 &6.08 &4.97 \\}{94.88 &94.9 &94.88 &94.87 &91.94 &92.58 &93.34 \\
93.22 &93.24 &93.22 &93.2 &89.92 &90.52 &91.29 \\
93.03 &93.02 &93.03 &92.99 &87.64 &89.05 &90.99 \\
79.93 &80.53 &79.93 &79.97 &63.72 &55.41 &56.59 \\}{73.79 &80.37 &73.79 &71.48 &66.36 &67.39 &79.21 \\
73.28 &79.26 &73.28 &70.87 &63.28 &63.94 &77.24 \\
62.23 &71.29 &62.23 &57.66 &53.57 &54.7 &69.92 \\
31.48 &42.37 &31.48 &19.45 &14.95 &13.65 &25.69 \\}{96.26 &96.24 &96.26 &96.24 &93.74 &94.15 &94.75 \\
94.93 &94.91 &94.93 &94.9 &91.77 &92.41 &93.32 \\
94.65 &94.66 &94.65 &94.62 &91.81 &92.16 &93.01 \\
84.33 &84.63 &84.33 &84.3 &78.79 &75.91 &75.71 \\}{72.09 &79.75 &72.09 &69.64 &63.9 &65.25 &81.69 \\
72.09 &79.27 &72.09 &69.7 &61.54 &62.44 &73.53 \\
60.48 &70.6 &60.48 &55.55 &49.83 &51.17 &71.68 \\
28.83 &52.36 &28.83 &16.11 &6.19 &4.09 &13.16 \\}{\ewtpos}

\myTable{96.76 &96.97 &96.76 &96.83 &90.68 &91.25 &93.58 \\
95.54 &95.77 &95.54 &95.6 &70.15 &70.94 &73.47 \\
96.27 &96.56 &96.27 &96.36 &89.42 &89.75 &92.3 \\
83.33 &84.39 &83.33 &83.28 &25.51 &25.49 &28.1 \\}{66.04 &73.18 &66.04 &65.9 &63.81 &64.93 &72.51 \\
67.93 &74 &67.93 &67.71 &45.73 &46.26 &51.49 \\
59.65 &68.86 &59.65 &59.42 &57.48 &57.22 &64.86 \\
24.79 &39.33 &24.79 &24.84 &4.38 &4.23 &5.88 \\}{97.05 &97.28 &97.05 &97.13 &90.39 &90.16 &91.12 \\
96.02 &96.28 &96.02 &96.09 &73.69 &73.29 &74.36 \\
96.41 &96.72 &96.41 &96.52 &88.76 &88.15 &89.17 \\
83.52 &84.23 &83.52 &83.45 &26 &25.66 &26.83 \\}{65.55 &74 &65.55 &64.83 &63.11 &64.57 &72.91 \\
67.98 &74.72 &67.98 &66.99 &46.26 &47.13 &53.98 \\
58.58 &69.55 &58.58 &57.58 &57.56 &57.49 &69.45 \\
19.9 &32.39 &19.9 &17.76 &3.17 &2.73 &4.85 \\}{97.1 &97.38 &97.1 &97.19 &87.84 &87.81 &90.61 \\
95.95 &96.26 &95.95 &96.03 &70.33 &70.64 &72.97 \\
96.53 &96.89 &96.53 &96.65 &86.78 &86.14 &88.58 \\
84.31 &84.97 &84.31 &84.22 &27.45 &26.16 &26.28 \\}{82.87 &86.15 &82.87 &83.15 &71.76 &73.37 &76.78 \\
81.28 &84.84 &81.28 &81.73 &53.33 &54.2 &56.97 \\
78.03 &82.28 &78.03 &78.1 &67.8 &68.39 &72.14 \\
48.84 &46.34 &48.84 &43.65 &7.08 &7.89 &10.71 \\}{97.42 &97.69 &97.42 &97.52 &90.91 &89.94 &90.79 \\
96.28 &96.57 &96.28 &96.36 &73.97 &72.6 &73.81 \\
96.89 &97.23 &96.89 &97 &89.97 &88.48 &89.04 \\
84.86 &85.52 &84.86 &84.89 &28.49 &27.98 &28.29 \\}{81.81 &86.47 &81.81 &82.28 &70.3 &72.18 &76.95 \\
80.15 &85.38 &80.15 &80.96 &53.85 &55.23 &60.07 \\
76.92 &83.06 &76.92 &77.2 &66.27 &67.16 &72.43 \\
47.99 &43.63 &47.99 &39.12 &5.29 &5.39 &8.41 \\}{\ptbpos}

\myTable{73.26 &73.01 &73.26 &72.13 &24.01 &25.54 &30.14 \\
68.67 &68.1 &68.67 &66.98 &21.84 &23.36 &28.31 \\
72.45 &72.27 &72.45 &71.24 &23.61 &25.19 &29.92 \\
67.79 &67.21 &67.79 &65.95 &21.87 &23.22 &28.09 \\}{50.96 &56.69 &50.96 &45.73 &10.05 &10.51 &17.27 \\
45.68 &49.8 &45.68 &37.65 &8.37 &8.59 &15.88 \\
49.57 &55.5 &49.57 &43.85 &9.56 &9.96 &16.7 \\
44.45 &47.9 &44.45 &35.42 &7.58 &7.85 &15.21 \\}{74.55 &74.71 &74.55 &73.35 &22.55 &24.54 &32.12 \\
69.69 &69.78 &69.69 &67.93 &20.46 &22.48 &30.97 \\
73.62 &73.9 &73.62 &72.34 &21.97 &24.03 &31.94 \\
68.71 &69.03 &68.71 &66.8 &19.83 &21.97 &30.75 \\}{51.5 &56.95 &51.5 &47.37 &10.43 &11.15 &20.23 \\
46.16 &49.7 &46.16 &39.35 &8.71 &9.23 &19.03 \\
50.22 &56.18 &50.22 &45.61 &10 &10.65 &19.97 \\
44.96 &47.62 &44.96 &37.16 &7.95 &8.47 &16.92 \\}{84.62 &83.72 &84.62 &83.86 &27.98 &29.11 &31.57 \\
81.01 &79.71 &81.01 &79.92 &26.1 &27.33 &30.2 \\
83.88 &82.93 &83.88 &83.07 &27.52 &28.71 &31.26 \\
80.26 &78.84 &80.26 &79.06 &25.64 &26.85 &29.72 \\}{59.81 &62.91 &59.81 &57.11 &13.01 &13.81 &18.76 \\
52.68 &54.74 &52.68 &48 &11.07 &11.73 &17.06 \\
58.01 &61.38 &58.01 &55 &12.4 &13.17 &18.42 \\
51.06 &52.91 &51.06 &45.66 &10.13 &10.92 &16.98 \\}{85.22 &84.57 &85.22 &84.45 &28.29 &29.49 &33.62 \\
81.56 &80.6 &81.56 &80.45 &25.87 &27.22 &32.11 \\
84.51 &83.81 &84.51 &83.67 &27.83 &29.08 &33.29 \\
80.86 &79.82 &80.86 &79.66 &25.79 &26.98 &31.84 \\}{59.58 &62.27 &59.58 &56.75 &12.62 &13.37 &19.51 \\
52.9 &54.48 &52.9 &48.37 &10.84 &11.33 &17.38 \\
57.8 &60.75 &57.8 &54.67 &12 &12.69 &19.42 \\
51.34 &52.71 &51.34 &46.17 &9.81 &10.3 &16.59 \\}{\ontonotessrl}

\myTable{92.57 &92.52 &92.57 &92.5 &56.3 &55.34 &57.17 \\
91.69 &91.62 &91.69 &91.6 &54.88 &54.4 &56.41 \\
86.68 &86.58 &86.68 &86.51 &50.93 &50.48 &52.67 \\
81.43 &80.92 &81.43 &80.86 &27.27 &26.59 &28.59 \\}{67.48 &71.61 &67.48 &65.7 &24.69 &25.9 &36.04 \\
67.18 &71.42 &67.18 &65.42 &24.76 &25.79 &35.6 \\
48.85 &46.89 &48.85 &42.99 &16.33 &16.54 &21.18 \\
50.29 &41 &50.29 &40.51 &5.15 &4.45 &5.78 \\}{94.35 &94.3 &94.35 &94.29 &60.85 &60.22 &61.35 \\
93.39 &93.32 &93.39 &93.31 &61.16 &59.97 &60.95 \\
89.31 &89.28 &89.31 &89.19 &58.12 &58.04 &59.7 \\
84.4 &83.9 &84.4 &83.77 &25.91 &25.06 &26.84 \\}{66.42 &70.43 &66.42 &64.86 &24.56 &25.24 &34.92 \\
66.28 &70.45 &66.28 &64.92 &25.12 &25.55 &34.52 \\
48.91 &49.07 &48.91 &43.63 &16.41 &16.19 &25.73 \\
50.81 &41.09 &50.81 &41.97 &5.28 &4.63 &5.94 \\}{94.69 &94.7 &94.69 &94.67 &60.22 &58.46 &60.06 \\
93.75 &93.78 &93.75 &93.73 &59.43 &57.57 &59.23 \\
90.29 &90.23 &90.29 &90.2 &55.56 &54.35 &54.92 \\
84.88 &84.39 &84.88 &84.38 &27.83 &27.84 &31.79 \\}{74.19 &78.18 &74.19 &72.37 &25.59 &28.03 &37.66 \\
66.97 &71.62 &66.97 &65.21 &23.61 &25.13 &35.41 \\
48.52 &46.85 &48.52 &42.36 &15.14 &15.69 &20.79 \\
50.15 &42.11 &50.15 &39.88 &5.13 &4.43 &6.05 \\}{95.76 &95.78 &95.76 &95.74 &64.08 &62.47 &62.66 \\
94.92 &94.93 &94.92 &94.89 &63.05 &61.95 &62.42 \\
92.06 &92.1 &92.06 &92 &61.89 &61.35 &62.13 \\
86.97 &86.58 &86.97 &86.5 &26.86 &26.03 &27.2 \\}{73.99 &77.74 &73.99 &72.53 &27.62 &29.28 &35.94 \\
66.11 &69.82 &66.11 &64.83 &25.72 &26.08 &34.81 \\
48.5 &46.66 &48.5 &43.6 &16.94 &16.71 &21.41 \\
50.54 &40.27 &50.54 &42.47 &5.33 &4.75 &5.51 \\}{\conllchunking}

\myTable{55.72 &58.19 &55.72 &53.95 &46.23 &47.33 &58.93 \\
55.14 &56.51 &55.14 &53.21 &45.14 &45.98 &53.18 \\
55.67 &58.11 &55.67 &53.89 &46.16 &47.26 &58.86 \\
55.1 &56.43 &55.1 &53.16 &45.1 &45.93 &53.13 \\}{22.56 &35.55 &22.56 &17.02 &12.4 &11.99 &30.13 \\
22.37 &34.59 &22.37 &16.7 &11.82 &11.32 &29.13 \\
22.59 &35.57 &22.59 &17.05 &12.4 &12 &30.13 \\
22.39 &34.57 &22.39 &16.72 &11.82 &11.33 &29.13 \\}{51.6 &57.75 &51.6 &49.17 &38.55 &40.12 &53.07 \\
50.93 &56.73 &50.93 &48.28 &37.69 &39.12 &52.26 \\
51.58 &57.73 &51.58 &49.15 &38.53 &40.09 &53.05 \\
50.88 &56.65 &50.88 &48.2 &37.62 &39.03 &52.18 \\}{24.48 &26.19 &24.48 &19.85 &16.34 &14.81 &21.93 \\
24.4 &26.48 &24.4 &19.74 &15.99 &14.46 &22.07 \\
24.48 &26.2 &24.48 &19.86 &16.34 &14.81 &21.93 \\
24.35 &26.32 &24.35 &19.65 &15.92 &14.36 &21.88 \\}{65.51 &68.01 &65.51 &65.45 &55.96 &58.81 &66.14 \\
65.07 &67.57 &65.07 &64.99 &55.1 &58.05 &65.58 \\
65.48 &67.96 &65.48 &65.4 &55.9 &58.76 &66.1 \\
65.04 &67.54 &65.04 &64.96 &55.07 &58.03 &65.57 \\}{26.06 &33.32 &26.06 &20.1 &16.2 &14.59 &28.28 \\
25.99 &30.78 &25.99 &19.91 &15.71 &14.05 &24.99 \\
26.05 &31.35 &26.05 &20.06 &16.16 &14.5 &25.65 \\
26.01 &30.78 &26.01 &19.93 &15.72 &14.07 &24.99 \\}{64.3 &63.08 &64.3 &63.18 &56.44 &55.74 &56.23 \\
63.84 &62.55 &63.84 &62.68 &55.6 &55.01 &55.71 \\
64.29 &63.07 &64.29 &63.17 &56.43 &55.73 &56.21 \\
63.8 &62.51 &63.8 &62.64 &55.56 &54.97 &55.67 \\}{26.39 &29.66 &26.39 &24.09 &19.98 &18.03 &26.62 \\
26.08 &29.57 &26.08 &23.84 &19.56 &17.6 &26.28 \\
26.4 &29.66 &26.4 &24.1 &19.98 &18.04 &26.62 \\
26.03 &29.55 &26.03 &23.81 &19.5 &17.55 &26.24 \\}{\semeval}

\myTable{71.74 &70.92 &71.74 &70.65 &50.14 &50.69 &55.16 \\
66.78 &65.8 &66.78 &65.38 &47.43 &48.02 &52.89 \\
68.6 &67.66 &68.6 &67.29 &47.33 &48.08 &53.3 \\
62.17 &61.01 &62.17 &60.45 &34.44 &33.64 &41.63 \\}{46.2 &45 &46.2 &41.1 &25.21 &26.16 &37.8 \\
42.8 &40.21 &42.8 &36.24 &24.08 &25.11 &36.56 \\
42.66 &40.51 &42.66 &36.71 &19.04 &20.14 &33.77 \\
38.15 &34.68 &38.15 &30.24 &9.32 &8.07 &16.28 \\}{73.1 &71.96 &73.1 &72.02 &49.71 &50.23 &53.94 \\
67.75 &66.53 &67.75 &66.44 &46.9 &47.35 &51.54 \\
69.93 &68.66 &69.93 &68.68 &47 &47.51 &51.9 \\
62.81 &61.51 &62.81 &61.3 &36.68 &34.32 &38.59 \\}{46.91 &46.39 &46.91 &41.93 &23.97 &25.48 &39.06 \\
43.17 &41.7 &43.17 &37.17 &21.61 &22.3 &32.79 \\
43.14 &42.08 &43.14 &37.59 &18.65 &20.12 &34.72 \\
38.21 &37 &38.21 &31.55 &8.58 &8.94 &17.41 \\}{79.05 &78.66 &79.05 &78.64 &56.41 &56.73 &59.76 \\
74.61 &74.21 &74.61 &74.11 &54.41 &54.39 &57.87 \\
76.42 &76.03 &76.42 &75.97 &53.74 &54.19 &57.7 \\
70.55 &70.18 &70.55 &69.99 &42.26 &41.27 &46.33 \\}{60.43 &62.04 &60.43 &58.97 &37.19 &37.03 &46.2 \\
55.02 &56.43 &55.02 &53.11 &34.31 &33.85 &42.4 \\
56.19 &57.73 &56.19 &54.44 &31.32 &31.32 &42.71 \\
49 &49.41 &49 &46.26 &16.76 &16.4 &24.9 \\}{79.63 &79.25 &79.63 &79.2 &58.05 &59.1 &63.74 \\
75.1 &74.71 &75.1 &74.58 &55.99 &57.27 &62.31 \\
77.03 &76.66 &77.03 &76.55 &55.91 &56.74 &61.36 \\
71.05 &70.72 &71.05 &70.47 &48.83 &49.68 &54.69 \\}{60.62 &62.44 &60.62 &58.39 &37.04 &37.55 &48.01 \\
55.36 &57.22 &55.36 &52.43 &32.58 &32.94 &43.09 \\
56.41 &58.17 &56.41 &53.71 &32.02 &32.58 &44.5 \\
49.44 &50.15 &49.44 &45.17 &16.41 &16.34 &27.21 \\}{\ontonotesconst}

\myTable{75.96 &75.4 &75.96 &75.12 &50.83 &52.5 &57.16 \\
69.61 &70.29 &69.61 &68.89 &48.06 &50.04 &56.3 \\
75.86 &75.56 &75.86 &75.06 &50.16 &51.91 &56.83 \\
69.35 &70.6 &69.35 &68.83 &45.97 &47.93 &54.46 \\}{46.15 &49.36 &46.15 &43.33 &22.84 &22.94 &33.04 \\
33.25 &37.68 &33.25 &29.81 &19.49 &19.22 &27.1 \\
45.83 &49.78 &45.83 &42.92 &21.84 &21.96 &32.96 \\
32.6 &37.62 &32.6 &29.06 &17.31 &16.72 &24.09 \\}{78.12 &77.01 &78.12 &77.06 &51.64 &52.85 &56.77 \\
71.94 &71.92 &71.94 &70.89 &49.09 &50.42 &56.18 \\
78.15 &77.22 &78.15 &77.11 &51.44 &52.62 &56.8 \\
71.78 &72.29 &71.78 &70.89 &47.57 &49.2 &55.58 \\}{45.11 &48.86 &45.11 &42.95 &21.93 &22.49 &32.52 \\
32.22 &37.46 &32.22 &29.83 &18.68 &19.23 &27.65 \\
44.72 &48.91 &44.72 &42.49 &20.66 &21.11 &29.54 \\
31.36 &38.01 &31.36 &28.99 &16.41 &16.44 &24.48 \\}{86.37 &86.33 &86.37 &85.92 &60.63 &62.72 &68.44 \\
81.11 &81.03 &81.11 &80.41 &57.95 &59.93 &66.04 \\
85.97 &85.91 &85.97 &85.49 &60.21 &62.18 &67.87 \\
80.57 &80.48 &80.57 &79.85 &56.85 &58.44 &64.37 \\}{58.11 &59.32 &58.11 &56.75 &29.34 &29.62 &34.41 \\
44.09 &45.89 &44.09 &42.33 &25.72 &25.82 &30.83 \\
56.94 &58.32 &56.94 &55.56 &28.2 &28.42 &33.39 \\
42.43 &44.21 &42.43 &40.55 &22.91 &22.68 &26.82 \\}{87.53 &87.06 &87.53 &86.77 &60.99 &62.5 &67.11 \\
82.24 &81.81 &82.24 &81.17 &58.78 &59.79 &64.32 \\
87.11 &86.63 &87.11 &86.31 &60.45 &61.83 &66.35 \\
81.63 &81.26 &81.63 &80.54 &57.03 &57.61 &62.35 \\}{57.97 &59.52 &57.97 &57.37 &29.71 &29.32 &32.29 \\
43.83 &46.42 &43.83 &43.15 &26.15 &25.66 &29.14 \\
56.88 &58.53 &56.88 &56.28 &28.72 &28.17 &31.03 \\
42.35 &45.03 &42.35 &41.64 &23.72 &23.08 &26.28 \\}{\ewtsyndepcls}

\myTable{86.57 &86.11 &86.57 &86.08 &72.54 &74.15 &79.31 \\
79.71 &78.91 &79.71 &78.75 &70.48 &71.85 &77.05 \\
86.45 &85.93 &86.45 &85.89 &71.45 &73.05 &78.39 \\
78.58 &77.68 &78.58 &77.39 &67.17 &68.32 &74.39 \\}{52.58 &54.29 &52.58 &50.88 &37.28 &36.36 &44.67 \\
37.33 &39 &37.33 &34.53 &34.54 &32.69 &39.03 \\
52.07 &53.79 &52.07 &50.43 &34.67 &33.79 &42.02 \\
33.59 &35.52 &33.59 &30.81 &28.84 &27.21 &33.01 \\}{87.44 &86.88 &87.44 &86.92 &74.17 &74.74 &77.47 \\
80.42 &79.45 &80.42 &79.43 &71.98 &72.14 &74.89 \\
87.19 &86.51 &87.19 &86.58 &73 &73.41 &76.22 \\
79.19 &77.68 &79.19 &77.86 &68.13 &68.18 &71.3 \\}{52.12 &53.81 &52.12 &50.79 &36.54 &36.11 &43.56 \\
36.59 &37.58 &36.59 &34.25 &33.55 &32.42 &39.46 \\
51.74 &54 &51.74 &50.38 &34.36 &33.8 &42.68 \\
32.96 &34.94 &32.96 &30.52 &27.9 &26.89 &35.04 \\}{93.15 &92.99 &93.15 &92.85 &78.62 &80.1 &84.96 \\
88.31 &87.98 &88.31 &87.69 &76.55 &77.72 &82.47 \\
92.7 &92.47 &92.7 &92.34 &77.52 &79.12 &84.12 \\
86.85 &86.31 &86.85 &86.03 &72.83 &73.94 &79.09 \\}{65.15 &67.81 &65.15 &63.57 &44.11 &44.99 &53.27 \\
49.54 &54.36 &49.54 &47.27 &41.24 &41.42 &49.99 \\
63.62 &65.92 &63.62 &61.8 &41.67 &42.16 &49.42 \\
44.12 &47.41 &44.12 &41.34 &34.85 &34.75 &41.41 \\}{93.72 &93.56 &93.72 &93.44 &81.38 &81.41 &84.05 \\
88.86 &88.56 &88.86 &88.32 &79.49 &79.19 &81.58 \\
93.24 &93.02 &93.24 &92.92 &80.39 &80.42 &83.2 \\
87.42 &86.9 &87.42 &86.7 &75.49 &75.29 &78.19 \\}{64.87 &67.28 &64.87 &63.59 &43.79 &44.39 &52.22 \\
49.27 &53.6 &49.27 &47.35 &40.38 &40.19 &48.11 \\
63.41 &65.66 &63.41 &61.96 &40.99 &41.16 &48.22 \\
44 &46.93 &44 &41.61 &33.95 &33.43 &39.13 \\}{\ptbsyndepcls}
\end{document}
